# Supplementary material for: Low spin wave damping in the insulating chiral magnet Cu$_{2}$OSeO$_{3}$
Source: arXiv:1705.03416 ancillary file (2017-05-09)
Supplement: Supplementary file 1 [file Damping_CuOSeO_supp20170504.pdf]

# Supplemental Information to Low spin wave damping in the insulating chiral magnet $Cu_2OSeO_3$

I. Stasinopoulos,[1,*] S. Weichselbaumer,[1] A. Bauer,[2] J. Waizner,[3]
H. Berger,[4] S. Maendl,[1] M. Garst,[3,5] C. Pfleiderer,[2] and D. Grundler[6,†]

[1] *Physik Department E10, Technische Universität München, D-85748 Garching, Germany*
[2] *Physik Department E51, Technische Universität München, D-85748 Garching, Germany*
[3] *Institute for Theoretical Physics, Universität zu Köln, D-50937 Köln, Germany*
[4] *Institut de Physique de la Matière Complexe, École Polytechnique Fédérale de Lausanne, 1015 Lausanne, Switzerland*
[5] *Institut für Theoretische Physik, Technische Universität Dresden, D-01062 Dresden, Germany*
[6] *Institute of Materials and Laboratory of Nanoscale Magnetic Materials and Magnonics (LMGN), École Polytechnique Fédérale de Lausanne (EPFL), Station 12, 1015 Lausanne, Switzerland*

(Dated: May 9, 2017)

## COPLANAR WAVEGUIDES

Figure 1 shows sketches illustrating the two different CPWs used in out studies. Table I summarizes the corresponding parameters for the two CPWs.

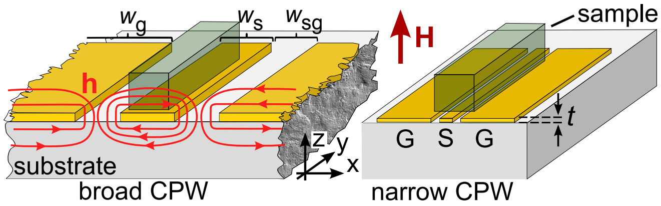


FIG. 1. Sample-mounted broad and narrow CPWs with signal (S) line width $w_s = 1$ mm and $20\,\mu$m, respectively (not to scale). The static field **H** is applied perpendicular to the CPW plane and the rf field **h** circulates around the conduction lines.

| CPW | $w_s$ ($\mu$m) | $w_g$ ($\mu$m) | $w_{sg}$ ($\mu$m) | $t$ ($\mu$m) | metallization |
|---|---|---|---|---|---|
| broad | 1000 | 5000 | 330 | 50 | Cu |
| narrow | 20 | 295 | 12.4 | 0.12 | Cr/Au |

TABLE I. Dimensions of the coplanar waveguides used in this study.

## CUBIC ANISOTROPY

For the description of cubic anisotropy, we consider the following Hamiltonian density.

$$\mathcal{H} = \frac{\mu_0}{2}\mathbf{M}\cdot\underline{N}\cdot\mathbf{M} + \frac{K}{M_s^4}\left(M_x^4 + M_y^4 + M_z^4\right) - \mathbf{B}_{ext}\cdot\mathbf{M} \quad (1)$$

With the demagnetization tensor $\underline{N}$, the anisotropy constant $K$, the saturation magnetization $M_s = |\mathbf{M}|$ and the externally applied magnetic flux density $\mathbf{B}_{ext}$. Assuming a rectangular prism with **H** parallel to a main axis and $N_x + N_y + N_z = 1$, the demagnetization tensor components for our samples were estimated as $N_x = 0.40$, $N_y = 0.07$, and $N_z = 0.53$ [1]. Taking cubic anisotropy additionally into account, we get [2]

$$\omega = \gamma\sqrt{\left(4\frac{K}{M_s} - \left(B_{\text{ext}} + \mu_0 M_s\left(N_x - N_z\right)\right)\right)\left(4\frac{K}{M_s} - \left(B_{\text{ext}} + \mu_0 M_s\left(N_y - N_z\right)\right)\right)} \quad (2)$$

and

$$\omega = \gamma\sqrt{\left(\frac{8}{3}\frac{K}{M_s} + \left(B_{\text{ext}} + \mu_0 M_s\left(N_x - N_z\right)\right)\right)\left(\frac{8}{3}\frac{K}{M_s} + \left(B_{\text{ext}} + \mu_0 M_s\left(N_y - N_z\right)\right)\right)} \quad (3)$$

for $\mathbf{H} \parallel \langle 100\rangle$ and $\mathbf{H} \parallel \langle 111\rangle$, respectively. Note that the Landé factor $g = 2.14$ is included in the gyromagnetic factor $\gamma$.

In Fig. 2, we show the main peak positions $f_r$ recorded with the broad CPW for $\mathbf{H} \parallel \langle 100\rangle$ and $\mathbf{H} \parallel \langle 111\rangle$ at 5 K (cf. Fig. 1 of the main text). We compare this to our

calculation by fitting the value of the anisotropy constant and obtain $K = (-0.6 \pm 0.1) \cdot 10^3$ J/m$^3$. The error corresponds to 5% deviation between theory and experiment, i.e. approximately half the data point symbol size. We also plot the Kittel formula [3] as the gray line, where the cubic anisotropy is neglected.

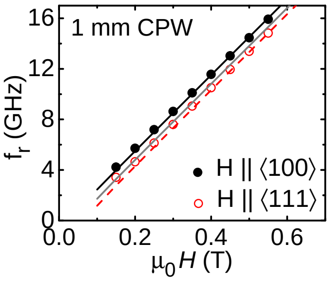


FIG. 2. Comparison of data recorded with the broad CPW and theoretical calculation including cubic anisotropy at 5 K. Black and red dashed lines show the expected resonance frequency for $\mathbf{H} \parallel \langle 100\rangle$ and $\mathbf{H} \parallel \langle 111\rangle$, respectively. The gray line corresponds to the Kittel formula.

## COMPARISON WITH OTHER WORK

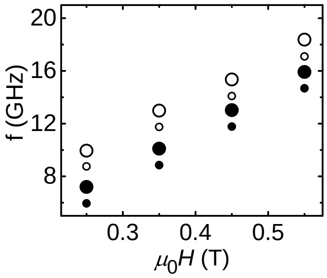


FIG. 3. Open and filled symbols represent theoretical and experimental data following Ref. [4] and Fig. 3 (a) in the main text, respectively. Large and small symbols indicate the eigenfrequencies of the uniform mode and standing spin wave, respectively.

In Fig. 3, experimental data (filled symbols) are compared to calculated eigenfrequencies (open symbols) obtained from the spin wave dispersion of Ref. [4]. For consistency, we multiplied our value for the anisotropy constant $K$ by $-2/S^4$, with $S = 0.48$, prior to performing the calculation of Ref. [4]. We considered $M_s = 0.5\,\mu_B/\mathrm{Cu}^+$ and $\mu_0 H_{c2}$=0.076 T at 5 K. Taking this into account, our value for $K$ at 5 K is approximately 3 times higher than the value reported at 30 K in Ref. [4]. Big and small circles show the frequency $f_{\mathrm{FMR}}$ and $f(k = \pi/d)$, respectively, where $d = 0.3$ mm is the sample thickness along $\mathbf{k}$.

In our work, we analyze and discuss data obtained at $\mu_0 H > 0.2$ T with $H$ being larger than $(N_z + N_x N_y/N_z)M_s$ where $N_x, N_y, N_z$ are the components of the demagnetization tensor. Following Ref. [2], the frequency $f_{\mathrm{FMR}}$ of ferromagnetic resonance (FMR), i.e., uniform precession, lies within the range for magnetostatic spin waves with a wave vector $k \neq 0$ considered in this work. In principle, the relaxation time $\tau_k$ of spin waves is different from $\tau_{\mathrm{FMR}}^{-1} = 2\pi\alpha_{\mathrm{intr}} f_{\mathrm{FMR}}$ attributed to the uniform FMR mode. Following Ref. [5], one finds $\tau_k^{-1} = \tau_{\mathrm{FMR}}^{-1}(f_{\mathrm{FMR}}^2 + f_{\mathrm{r}}^2)/2 f_{\mathrm{FMR}} f_{\mathrm{r}}$ for magnetostatic volume waves. When evaluating damping parameters $\alpha$ from spin waves we consider resonance frequencies $f_{\mathrm{r}}$ that are close to $f_{\mathrm{FMR}}$. In this case, $\tau_k \approx \tau_{\mathrm{FMR}}$ [5] and the evaluated Gilbert parameter $\alpha$ is a good estimate for $\alpha_{\mathrm{intr}}$. If spin-wave frequencies deviate from $f_{\mathrm{FMR}}$ the parameter $\alpha$ is larger than $\alpha_{\mathrm{intr}}$ and thereby a conservative estimate. Very recently, the Gilbert damping parameters of a series of standing magnetostatic spin wave modes in YIG were analyzed in detail and indeed provided values consistent with $\alpha_{\mathrm{intr}}$ extracted from FMR [6]. Similar to Ref. [6] our bulk ferrimagnet does not seem to experience radiative damping [7].

Note that the spin-wave propagation in a nonmetallized rectangular rod has no strict analytical solution [2] and the dispersion relation taken from Ref. [4] models a platelet instead of a rod. This explains the remaining discrepancy between closed and open symbols in absolute frequencies. The frequency splitting $\delta f$ is correctly modelled.

We note that Kobets *et al.* attributed sharp features to nonlinear parametric resonances induced by a nonuniformity [8], possibly due to an inhomogeneous internal field [9]. But, even below the threshold power for nonlinear excitation, the authors of Ref. [8] detected a substructure.

## ADDITIONAL LINEWIDTH DATA

The saturation magnetization in the unit cell does not vary significantly with the crystallographic orientation [10]. In Fig. 4 we show the extracted field and frequency linewidths, $\Delta H$ and $\Delta f$, respectively, upon which we determined the parameters shown in Fig. 3 (a)-(d) of the main text.

In Fig. 5 we show additional data recorded on a third sample with dimensions $0.5 \times 0.5 \times 3\,\mathrm{mm}^3$ and $\mathbf{H} \parallel \langle 100\rangle$ using the broad CPW. The fitted linewidths $\Delta f$ (after re-scaling with the factor $\sqrt{3}$) yield $\alpha_{\mathrm{intr}}$ $=(3.1 \pm 0.3)\times 10^{-3}$, in agreement with the value $(3.7 \pm 0.4)\times 10^{-3}$ presented in the main text.

We now discuss results regarding the sharp peaks obtained using the narrow CPW. In Fig. 6 (a) we replot the data shown in Fig. 1(a) [and in the inset of Fig. 4(b)] of the main text. We fit the peak labelled #4. Note that there is another peak of similar intensity (red

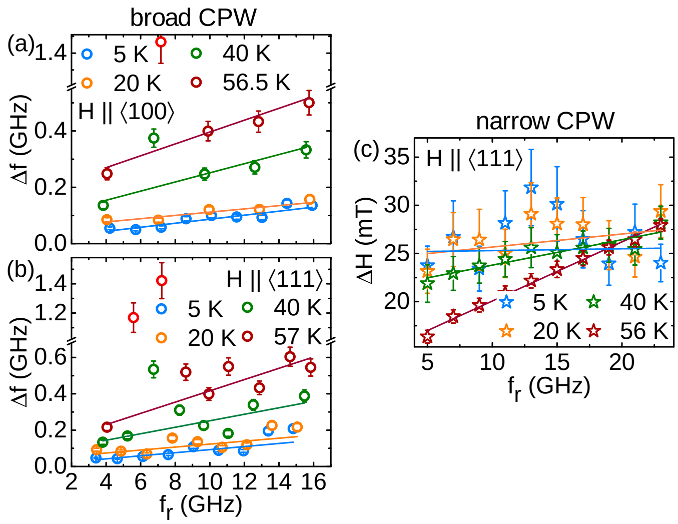


FIG. 4. Temperature and frequency dependent linewidth for different field orientations and CPWs. Linear fits to the data are shown. The red data points in panels (a),(b) have been excluded from the linear fit, because of the presence of strong cable resonances in the spectra, which distort the lineshape.

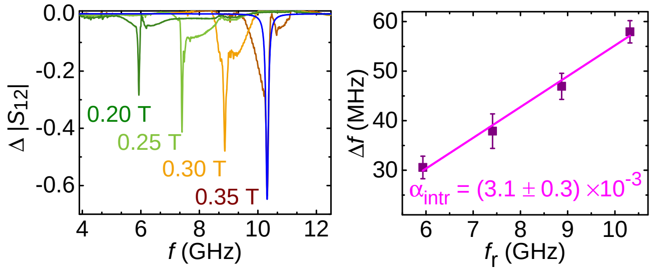


FIG. 5. (a) Spectra obtained from a third sample with $\mathbf{H} \parallel \langle 100\rangle$ at 0.85 T and 5 K using the broad CPW. An exemplary Lorentz fit curve is shown in blue. (b) Frequency dependency of the linewidth $\Delta f$ (symbols). The slope of the linear fit (magenta line) following Eq. (2) of the main text reflects the intrinsic damping parameter $\alpha_{\mathrm{intr}}$.

arrow) to the left. The rescaled linewidths $\Delta f$ obtained from spectra recorded at different fields [Fig. 6 (b)] do not scale linearly with the resonance frequency $f_r$. We attribute this fact along with the relatively large linewidth to the presence of further sharp peaks around 23.5 GHz that were not resolved.

We also summarize the rescaled linewidths obtained from a fit to the sharp peak #1 in Fig. 6 (c). A linear fit yields $\alpha_{\mathrm{intr}} = (2.6 \pm 0.1) \times 10^{-4}$. There is a discrepancy of $\alpha_{\mathrm{intr}}$ obtained from the sharp peaks in the case $\mathbf{H} \parallel \langle 111\rangle$ compared to the value $\alpha_{\mathrm{intr}} = (9.9 \pm 4.1) \times 10^{-5}$, which was obtained when $\mathbf{H} \parallel \langle 100\rangle$ (see main text). We attribute this to field-dragging contributions from a misalignment of $\mathbf{H}$ with the hard axis $\langle 111\rangle$. Finally, we note that the limited signal amplitude of the sharp peaks #2, #3 for $\mathbf{H} \parallel \langle 100\rangle$ in Fig. 5 (a) of the main text yields

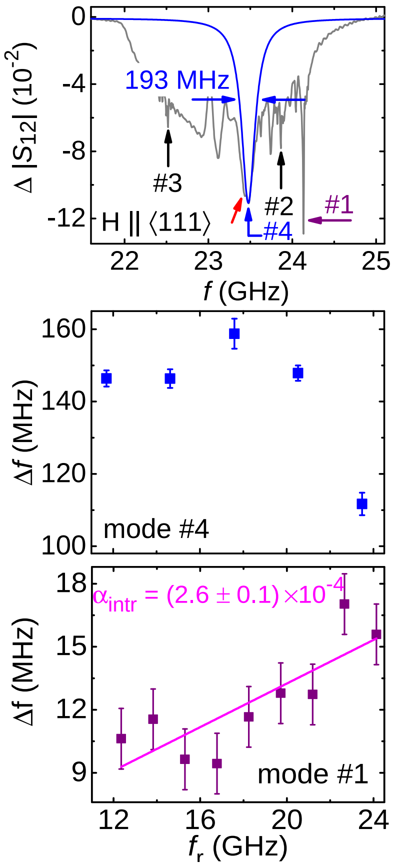


FIG. 6. (a) Sharp modes for $\mathbf{H} \parallel \langle 111\rangle$ at 5 K using the narrow CPW. An exemplary Lorentz fit curve of mode #4 is shown in blue. (b), (c) Frequency dependency of the linewidth $\Delta f$ obtained from modes #4 and #1, respectively. For the latter, we extract $\alpha_{\mathrm{intr}}$ from the slope of a linear fit to the data (magenta line).

untrustworthy fit results. Therefore, we concentrated on mode #1, which was best resolved.

* Electronic mail: i.stasinopoulos@ph.tum.de
† Electronic mail: dirk.grundler@epfl.ch

[1] A. Aharoni, J. Appl. Phys. **83**, 3432 (1998).
[2] A. G. Gurevich and G. A. Melkov, *Magnetization Oscillations and Waves* (CRC Press, 1996).
[3] C. Kittel, Phys. Rev. **73**, 155 (1948).
[4] S. Seki, Y. Okamura, K. Kondou, K. Shibata, M. Kubota, R. Takagi, F. Kagawa, M. Kawasaki, G. Tatara, Y. Otani, and Y. Tokura, Phys. Rev. B **93**, 235131 (2016).
[5] D. D. Stancil, *Theory of Magnetostatic Waves* (Springer, 1993).
[6] S. Klingler, H. Maier-Flaig, C. Dubs, O. Surzhenko, R. Gross, H. Huebl, S. T. B. Goennenwein, and M. Weiler, Applied Physics Letters **110**, 092409 (2017), http://dx.doi.org/10.1063/1.4977423.
[7] M. A. W. Schoen, J. M. Shaw, H. T. Nembach, M. Weiler, and T. J. Silva, Phys. Rev. B **92**, 184417 (2015).

[8] M. I. Kobets, K. G. Dergachev, E. N. Khatsko, A. I. Rykova, P. Lemmens, D. Wulferding, and H. Berger, Low Temp. Phys. **36** (2010).

[9] G. Zheng, M. PardaviHorvath, X. Huang, B. Keszei, and J. Vandlik, J. Appl. Phys. **79** (1996).

[10] T. Adams, A. Chacon, M. Wagner, A. Bauer, G. Brandl, B. Pedersen, H. Berger, P. Lemmens, and C. Pfleiderer, Phys. Rev. Lett. **108**, 237204 (2012).
